# Supplementary material for: Towards Personalized Review Summarization by Modeling Historical Reviews from Customer and Product Separately
Source: arXiv:2301.11682 source file (2023-01-27)
Supplement: Supplementary file 1 [file appendix.tex]

\input{results-all}
